# Supplementary material for: Why the World Reads Wikipedia: Beyond English Speakers
Source: arXiv:1812.00474 source file (2018-12-02)
Supplement: Supplementary file 1 [file 070appendix.tex]

%\appendix
%\section{Survey bias correction}
\section*{Acknowledgements}
\label{ap:ack}
Acknowledgements are omitted for double blind review.
